# Supplementary material for: AMASS: Archive of Motion Capture as Surface Shapes
Source: arXiv:1904.03278 source file (2019-04-05)
Supplement: Supplementary file 1 [file vposer.tex]

We demonstrate benefits of our dataset by taking a recent deep neural network based human pose prior (VPoser) \cite{nima2019} and show improvements in the originally reported metrics simply by re-training on AMASS.

To showcase impact of such a large human motion dataset we take a recent deep neural network architecture proposed as a human pose prior for 2D-to-3D human image lifting \cite{nima2019} and retrain it on AMASS. As their quantitative evaluations, the authors of \cite{nima2019} reported XX but we got YY and this is good.
